# Supplementary material for: Analytic $G_0W_0$ gradients based on a double-similarity transformation equation-of-motion coupled-cluster treatment
Source: arXiv:2510.23275 ancillary file (2025-10-27)
Supplement: Supplementary file 1 [file supp.pdf]

# Supporting Information for "Analytic $G_0W_0$ gradients based on a double-similarity transformation equation-of-motion coupled-cluster treatment"

Marios-Petros Kitsaras,[1, a)] Johannes Tölle,[2, b)] and Pierre-François Loos[1, c)]
[1)] *Laboratoire de Chimie et Physique Quantiques (UMR 5626), Université de Toulouse, CNRS, Toulouse, France*
[2)] *Department of Chemistry, University of Hamburg, 22761 Hamburg, Germany; The Hamburg Centre for Ultrafast Imaging (CUI), Hamburg 22761, Germany*

## I. POTENTIAL ENERGY CURVES FOR THE LIF MOLECULE AND ITS CATION

The potential energy curves are plotted for the LiF molecule at the ADC(2), CC2, $G_0W_0$, CCSD, CC3, and CCSDT levels of theory in Figs. 1, 2, 3, 4, 5, and 6. The cationic $^2\Pi$ (green) and $^2\Sigma$ (red) states were targeted starting from the lowest closed-shell state of the neutral system (blue) as described in the *Computational Details* section of the main paper. The cationic $^2\Pi$ state results from removing an electron from the HOMO $\pi$ orbital localized in the F atomic center. This orbital is not strongly contributing to the bond behavior, and as such, the resulting cation is weakly bound. On the other hand, the $^2\Sigma$ cationic state results from detaching an electron from the HOMO$-$1 bonding $\sigma$ orbital. This significantly affects the bonding behavior, and the resulting state is a non-bonding state with a shallow minimum.

As shown in Fig. 1, the ADC(2) approach overestimates the bond length of the cationic $^2\Pi$ state as compared to the rest of the predictions. Additionally, the expected degeneracy of the $^2\Pi$ and $^2\Sigma$ states in the limit of non-interacting atoms is strongly violated at this level of theory.

At the CC2 level (see Fig. 2), the quality of the reference wavefunction deteriorates rapidly for $R > 3.5$ Å, due to the perturbative character of the method and the emerging strong multiconfigurational character. This is seen by the energy diverging toward negative infinity. No physical energy minimum is observed for the cationic states, and no convergence for the CC2 amplitude equations could be achieved for $R > 4.0$ Å.

The predictions at the $G_0W_0$ (Fig. 3) and CCSD (Fig. 4) levels of theory are in agreement with each other. Both cationic states exhibit a physically expected behavior at these levels of theory. Moreover, the degeneracy of the $^2\Pi$ and $^2\Sigma$ states for large internuclear distances is violated by $\sim 0.1$ m$E_\text{h}$, which is within the accuracy expected by these levels of theory.

Results at the CC3 level of theory (Fig. 5) are rather unphysical for the cationic states. The minimum for the ground neutral state is 1.5762 Å at the CC3 level. This gives a 11.380 eV VIP for the $^2\Pi$ cationic state. A too shallow minimum is predicted for the $^2\Pi$ state at 3.8659 Å, significantly larger compared to the CCSDT results. The CC3 AIP (10.82 eV) is, however, predicted close to the CCSDT predictions. A significantly strong double-excitation character of both cationic states is observed for $R > 1.9$ Å, which is completely absent at the CCSDT level of theory. This finding, together with the strong violation of the expected degeneracy between the $^2\Pi$ and $^2\Sigma$ states by $\sim 0.1$ $E_\text{h}$ in the limit of non-interacting atoms, suggests that the CC3 predictions are not to be trusted. As such, they have not been used as a reference for this system. The failure of the CC3 approach to correctly describe the electron structure of the cationic system may arise due to the fact that we are unable to converge to the correct physical state at the IP-EOM-CC3 level of theory. Further investigation is beyond the scope of the current study.

Results at the CCSDT level of theory are presented in Fig. 6. They have been used for the LiF system instead of CC3 for the statistical analysis, and confirm the qualitative trends at the $G_0W_0$ and CCSD levels of theory.

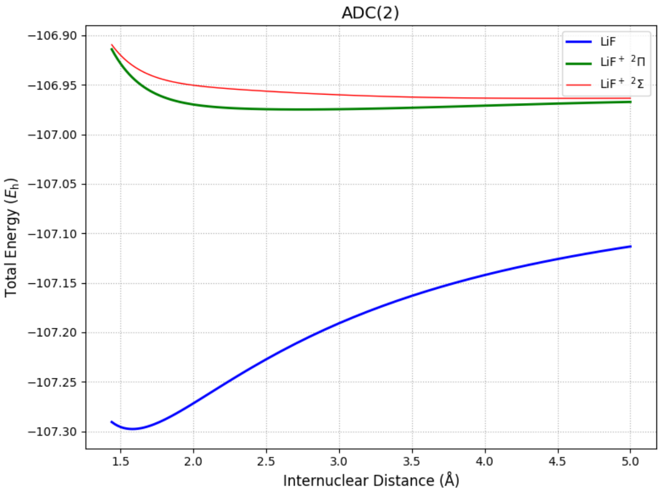


FIG. 1. Potential energy curves for the lowest closed-shell $^1\Sigma$ state (blue) of LiF and the $^2\Pi$ (green) and $^2\Sigma$ (red) states of $LiF^+$ at the ground-state and excited-state ADC(2) levels of theory respectively. All electrons were included for the calculation of correlation effects using the aug-cc-pVTZ basis set. Energy in $E_\text{h}$, distance in Å.

[a)] Electronic mail: kitsaras@irsamc.ups-tlse.fr
[b)] Electronic mail: johannes.toelle@uni-hamburg.de
[c)] Electronic mail: loos@irsamc.ups-tlse.fr

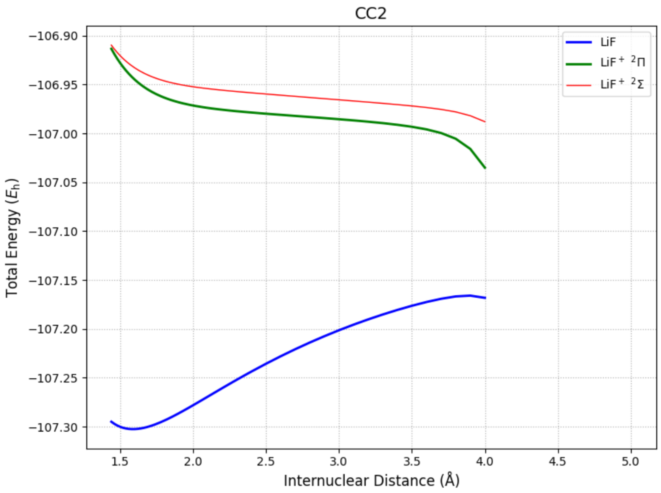


FIG. 2. Potential energy curves for the lowest closed-shell $^1\Sigma$ state (blue) of LiF and the $^2\Pi$ (green) and $^2\Sigma$ (red) states of LiF$^+$ at the CC2 and IP-EOM-CC2 levels of theory respectively. All electrons were included for the calculation of correlation effects using the aug-cc-pVTZ basis set. Energy in $E_\mathrm{h}$, distance in Å.

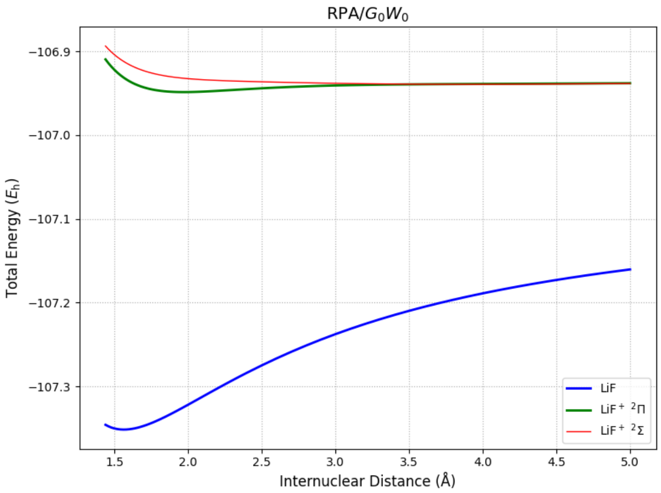


FIG. 3. Potential energy curves for the lowest closed-shell $^1\Sigma$ state (blue) of LiF and the $^2\Pi$ (green) and $^2\Sigma$ (red) states of LiF$^+$ at the RPA and $G_0W_0$ levels of theory respectively. All electrons were included for the calculation of correlation effects using the aug-cc-pVTZ basis set. Energy in $E_\mathrm{h}$, distance in Å.

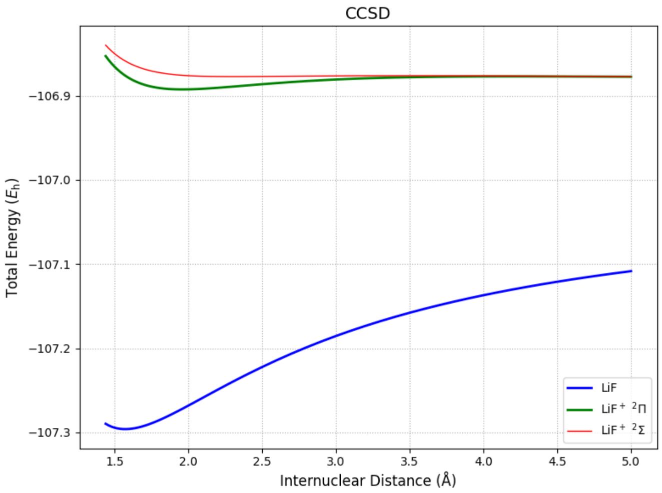


FIG. 4. Potential energy curves for the lowest closed-shell $^1\Sigma$ state (blue) of LiF and the $^2\Pi$ (green) and $^2\Sigma$ (red) states of LiF$^+$ at the CCSD and IP-EOM-CCSD levels of theory respectively. All electrons were included for the calculation of correlation effects using the aug-cc-pVTZ basis set. Energy in $E_\mathrm{h}$, distance in Å.

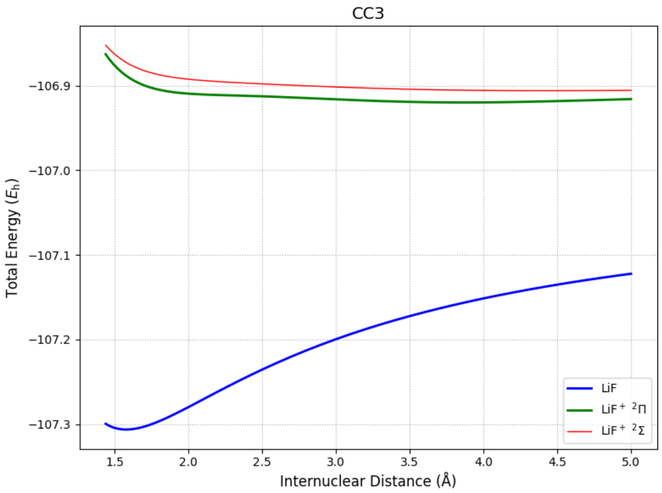


FIG. 5. Potential energy curves for the lowest closed-shell $^1\Sigma$ state (blue) of LiF and the $^2\Pi$ (green) and $^2\Sigma$ (red) states of LiF$^+$ at the CC3 and IP-EOM-CC3 levels of theory respectively. All electrons were included for the calculation of correlation effects using the aug-cc-pVTZ basis set. Energy in $E_\mathrm{h}$, distance in Å.

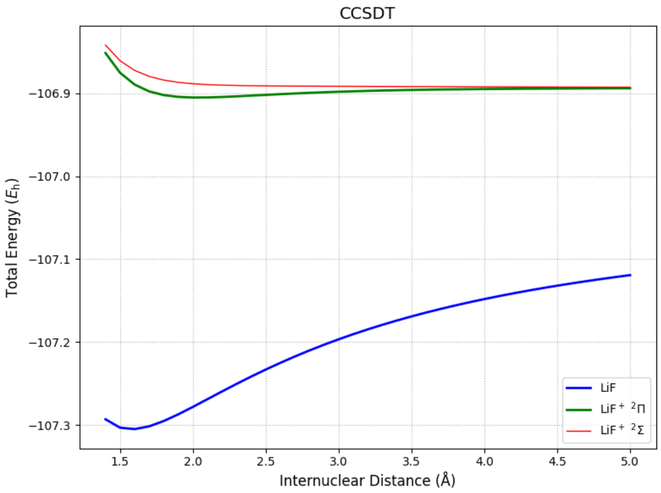


FIG. 6. Potential energy curves for the lowest closed-shell $^1\Sigma$ state (blue) of LiF and the $^2\Pi$ (green) and $^2\Sigma$ (red) states of $LiF^+$ at the CCSDT and IP-EOM-CCSDT levels of theory respectively. All electrons were included for the calculation of correlation effects using the aug-cc-pVTZ basis set. Energy in $E_\mathrm{h}$, distance in Å.

## II. COMPARISON OF CC3 AND CCSDT FOR HF, LIF, $N_2$ AND $F_2$

TABLE I. Vertical and adiabatic ionization potentials (in eV) using the aug-cc-pVTZ basis set. For the vertical IPs, the optimal geometry of the neutral molecule at the respective level of theory has been used. For the adiabatic IPs, the energy of the ionized state at the optimal geometry calculated at the respective level of theory has been subtracted from the optimal energy of the neutral molecule at the respective level of theory.

| | Vertical IPs | | Adiabatic IPs | |
|---|---|---|---|---|
| System | CC3 | CCSDT | CC3 | CCSDT |
| HF | 16.132 | 16.085 | 15.976 | 15.931 |
| LiF | 11.380 | 11.391 | 10.816 | 10.892 |
| $N_2$ | 16.851 | 16.979 | 16.461 | 16.661 |
| $F_2$ | 15.756 | 15.698 | 15.591 | 15.526 |

TABLE II. Interatomic distance (in Å) in the optimal geometry for the neutral $R_{\text{neu}}$ and cationic $R_{\text{cat}}$ linear molecules using the aug-cc-pVTZ basis set.

| | $R_{\text{neu}}$ | | $R_{\text{cat}}$ | |
|---|---|---|---|---|
| System | CC3 | CCSDT | CC3 | CCSDT |
| HF | 0.9196 | 0.9192 | 1.0075 | 1.0054 |
| LiF | 1.5783 | 1.5762 | 3.8659 | 2.0344 |
| $N_2$ | 1.1007 | 1.0993 | 1.1869 | 1.1727 |
| $F_2$ | 1.4137 | 1.4134 | 1.3145 | 1.3135 |

A comparison of the CC3 and CCSDT predictions is presented in Tables I and II for selected systems. For the non-problematic systems HF, $N_2$ and $F_2$ the absolute error of CC3 relative to CCSDT is 0.047 eV, 0.128 eV , 0.058 eV ,for the VIP 0.045 eV, 0.200 eV, 0.065 eV, for the AIP, 0.0004 Å, 0.0015 Å, 0.0028 Å for the neutral molecule and 0.0025 Å, 0.0142 Å, 0.0010 Å for the cation, respectively. These discrepancies are well below the typical errors observed for the other methods considered in the main text [ADC(2), CC2, $G_0W_0$, CCSD]. With the exception of LiF (see above), CC3 therefore constitutes a reliable reference method.
